# Supplementary material for: Parameter inference with estimated covariance matrices
Source: arXiv:1511.05969 source file (2016-01-05)
Supplement: Supplementary file 1 [file Appendix.tex]

\appendix

\section{Multiple estimates per simulation}
Often, one data vector will contains elements that can be arranged into groups that are independent and identically distributed (IID). This may arise from symmetry considerations, and in this case the simulated data will have the same property.  Given that, for a gaussian distribution, the information is in the mean and covariance, it is sensible to combine IID quantities, and effectively redefine the vector $\boX_i$:
\begin{equation}
\boX_i = 
\begin{pmatrix}
 x_1\\
.\\
.\\
.\\
x_p
\end{pmatrix}
= 
\begin{pmatrix}
 \frac{1}{n_1} \sum_{k = 1}^{n_1} \xi_{1,k}\\
.\\
.\\
.\\
 \frac{1}{n_p} \sum_{k = 1}^{n_p} \xi_{p,k}\\
\end{pmatrix}
\end{equation}
where the sums extend over IID components. This is, for example, useful for spherical harmonic coefficients of an expansion of statistically isotropic fields, where the $x_i$ correspond to different $\ell$-modes and the $\xi_{\ell, k}$ the different $m$-modes contributing to the $\ell$-modes.
